# Supplementary material for: Current rectification and ionic selectivity of alpha-hemolysin: Coarse-Grained Molecular Dynamics simulations
Source: arXiv:2201.12174 source file (2022-01-28)
Supplement: Supplementary file 1 [file Supplemental_Information_ACS_Nano.pdf]

# Supporting Information: Current rectification and ionic selectivity of $\alpha$-hemolysin: Coarse-Grained Molecular Dynamics simulations

Delphine Dessaux, Jérôme Mathé, Rosa Ramirez, and Nathalie Basdevant*

*Université Paris–Saclay, CNRS, Univ Evry, LAMBE, 91025, Évry–Courcouronnes, France*

E-mail: nathalie.basdevant@univ-evry.fr

## Supplemental Figures

The numbers of ions located within the stem of the different $\alpha$-hemolysin pores during each simulation were computed as explained in the supplemental information of our previous study[S1]. Moreover, for each electric field, we calculated the average number of ions in the stem from 1 to 1.5 $\mu$s of simulation which are represented on the figure S1 for the WT and K147N $\alpha$HL.

We observed different behaviors of the ion concentration inside the stem of $\alpha$-hemolysins related to their ionic selectivity. Indeed, as we can see on figure S1, the stem of a selective $\alpha$HL pore, such as the WT protein, contains less ions for the negative electric fields than for the positive ones whereas a non-selective pore, such as K147N, presents a constant average number of ions for all of the applied electric field.

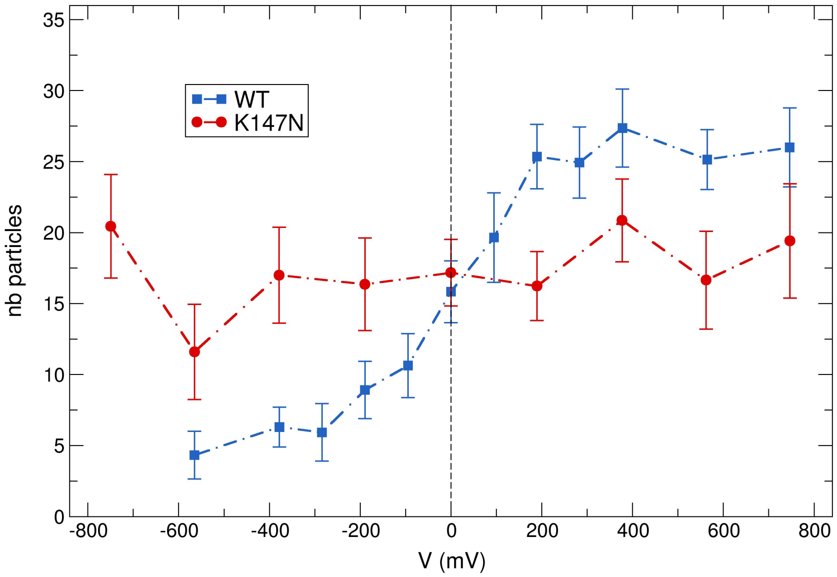


Figure S1: Average number of ions within the stem of the native pore (in blue) or the K147N $\alpha$-hemolysin (in red) as a function of applied voltage.

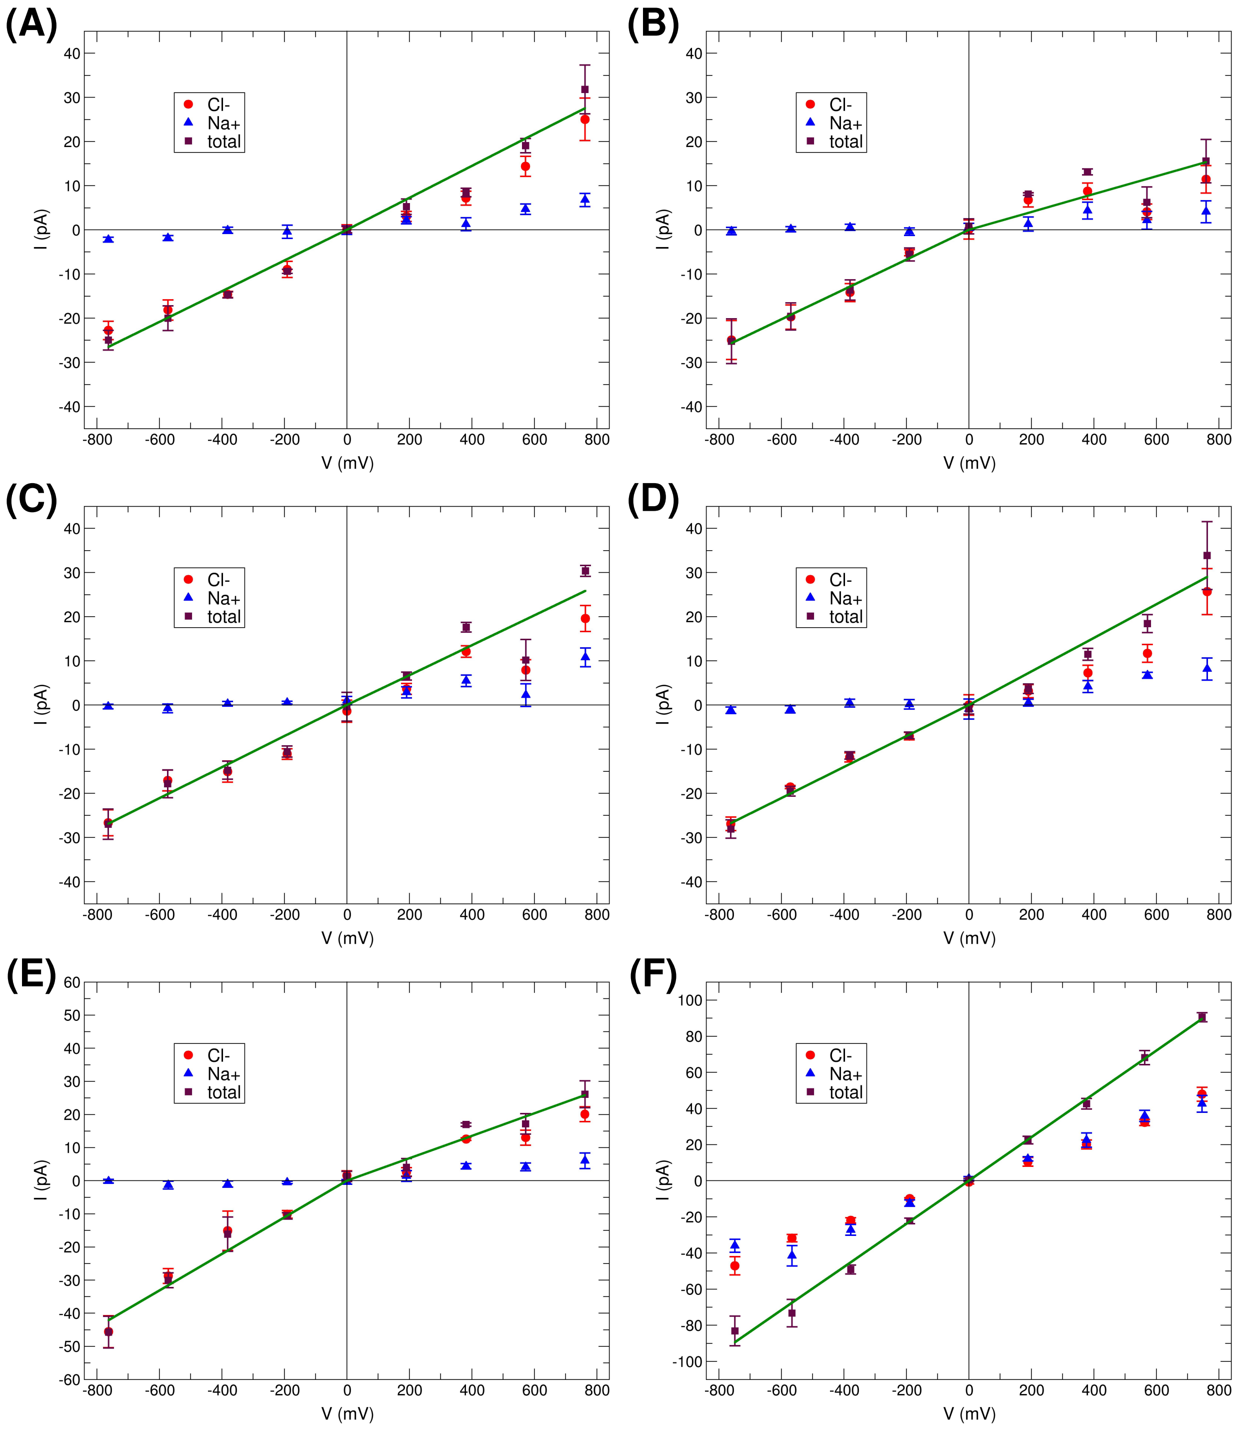


Figure S2: *IV* curves for the constrained $\alpha$HL with a neutral *trans* extremity: D127N-D128N-K131N* (A) and D127N* (B), or with a modified *trans* extremity: K131N* (C), D127N-D128N* (D) and D128N-K131N* (E), and the not-constrained E111N-K147N $\alpha$HL (F).

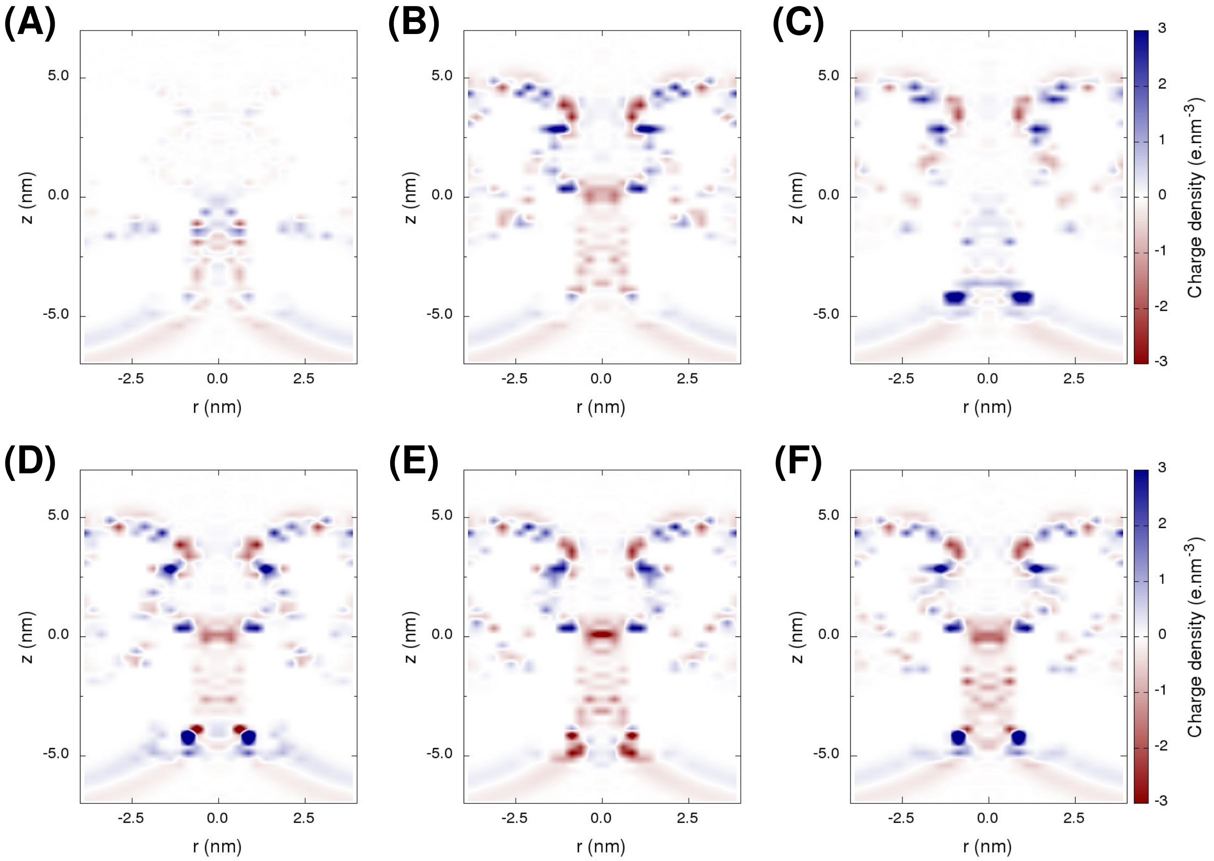


Figure S3: Density maps for the constrained neutral in the presence of a negative electric field $E_z = -0.03$ V/nm for the constrained neutral pore (A) and $\alpha$HL: D127N-D128N-K131N* (B), E111N-K147N (C), K131N* (D), D127N-D128N* (E) and D128N-K131N* (F).

# References

(S1) Basdevant, N.; Dessaux, D.; Ramirez, R. Ionic transport through a protein nanopore: a Coarse-Grained Molecular Dynamics Study. *Scientific Reports* **2019**, *9*, 15740.
